# Supplementary material for: SecVulEval: Benchmarking LLMs for Real-World C/C++ Vulnerability Detection
Source: arXiv:2505.19828 source file (2025-05-26)
Supplement: Supplementary file 1 [file appendix.tex]

\newpage
\appendix
\onecolumn
\noindent {\Large  \textbf{Appendix}}

Table of Contents: 
\begin{itemize}
    \item Appendix A: Limitation
    \item Appendix B: Details of prompts used in this paper
    \item Appendix C: Analysis of the model outputs for both detection and repair tasks
\end{itemize}

\section{Appendix A}
\label{appendix-a}
\section{Limitation}
\basim{Limitation section is required for NeurIPS}
While \textsc{SecVulEval} makes a significant step forward for Linux vulnerability research, there are some aspects that should be considered with our findings.

% \basim{kindly check if the internal/external classification is appropriate.}
\textit{Internal threats:} Output parsing failure is a common problem faced by researchers when working with LLMs because of their random behavior. This can affect the results as some LLM outputs might be excluded from analysis due to parsing errors. We mitigated this issue by explicitly prompting the models to output in json formats, along with few-shot examples. Moreover, we added an output post-processing stage to further reduce the error. Another source of threat is the prompts used for the study. LLMs' outputs can be strongly correlated with the input prompt. We kept a similar prompt with the same randomly selected few-shot examples across all models for fair comparisons, with slightly adjusting to specific model behaviors.

\textit{External threats:} NVD is a popular and long-standing source for vulnerability curation and it is possible that the models may have been pre-trained on specific vulnerability data. This may not accurately present the models' performances on future unseen data. Another potential discrepancy in models can arise from the implementation of the models. To mitigate this, we used all the models from HuggingFace\footnote{https://huggingface.co} using the \emph{transformers.pipeline} implementation, and official model generation examples from the HuggingFace model homepage. We left most of the hyperparameters to default settings as they have been thoroughly evaluated by the community and is standard.
\subsection{Function-level Vulnerability Detection}
\label{appndx:func_level_detection_scores}
Here, we provide the detailed scores of the function-level vulnerability detection scores from RQ1. GPT-4o outscores every other model in this task.
\begin{table}[H]
% \begin{adjustbox}{angle=90}
% Increases row height by 2.5 times
    \centering
      \caption{Function level vulnerability detection scores (\%) of the models. P, R, F1, and A in the header stand for Precision, Recall, F1-Score, and Accuracy, respectively.}
    \tiny
    \begin{tabular}{@{\hspace{0.8mm}}c@{\hspace{1mm}}|@{\hspace{0.8mm}}c@{\hspace{0.8mm}}@{\hspace{0.8mm}}c@{\hspace{0.8mm}}@{\hspace{0.8mm}}c@{\hspace{0.8mm}}@{\hspace{0.8mm}}c@{\hspace{1mm}}|@{\hspace{0.8mm}}c@{\hspace{0.8mm}} @{\hspace{0.8mm}}c@{\hspace{0.8mm}} @{\hspace{0.8mm}}c@{\hspace{0.8mm}} @{\hspace{0.8mm}}c@{\hspace{1mm}}|@{\hspace{0.8mm}}c@{\hspace{0.8mm}} @{\hspace{0.8mm}}c@{\hspace{0.8mm}} @{\hspace{0.8mm}}c@{\hspace{0.8mm}} @{\hspace{0.8mm}}c@{\hspace{1mm}}|@{\hspace{0.8mm}}c@{\hspace{0.8mm}} @{\hspace{0.8mm}}c@{\hspace{0.8mm}} @{\hspace{0.8mm}}c@{\hspace{0.8mm}} @{\hspace{0.8mm}}c@{\hspace{1mm}}|@{\hspace{0.8mm}}c@{\hspace{0.8mm}} @{\hspace{0.8mm}}c@{\hspace{0.8mm}} @{\hspace{0.8mm}}c@{\hspace{0.8mm}} @{\hspace{0.8mm}}c@{\hspace{1mm}}|@{\hspace{0.8mm}}c@{\hspace{0.8mm}} @{\hspace{0.8mm}}c@{\hspace{0.8mm}} @{\hspace{0.8mm}}c@{\hspace{0.8mm}} @{\hspace{0.8mm}}c@{ }}
    \hline
        \multirow{2}{*}{CWE Type} & \multicolumn{4}{c|@{\hspace{0.8mm}}}{CodeLlama} &  \multicolumn{4}{c|@{\hspace{0.8mm}}}{Deepseek-Coder} & \multicolumn{4}{c|@{\hspace{0.8mm}}}{Codestral} & \multicolumn{4}{c|@{\hspace{0.8mm}}}{StarCoder2} & \multicolumn{4}{c|@{\hspace{0.8mm}}}{Qwen2.5-Coder} & \multicolumn{4}{c}{GPT-4o} \\ \cline{2-25}
        ~ & P & R & F1 & A & P & R & F1 & A & P & R & F1 & A & P & R & F1 & A & P & R & F1 & A & P & R & F1 & A \\ \hline
        CWE-20 & 51.43 & 16.07 & 24.49 & 50.67 & \textbf{63.64} & 12.50 & 20.90 & 52.89 & 51.16 & 39.29 & 44.44 & 51.11 & 48.35 & 39.29 & 43.35 & 48.89 & 58.06 & 16.07 & 25.17 & 52.44 & 50.26 & \textbf{84.82} & \textbf{63.12} & 50.67 \\ \hline
        CWE-119 & 25.00 & 0.68 & 1.32 & 49.15 & 46.67 & 5.30 & 9.52 & 50.92 & \textbf{92.31} & 8.11 & 14.91 & 16.46 & 50.00 & 32.43 & 39.34 & 49.83 & 68.75 & 14.86 & 24.44 & 53.9 & 50.00 & \textbf{67.57} & \textbf{57.47} & 49.83 \\ \hline
        CWE-125 & 0.00 & 0.00 & 0.00 & 50.68 & 47.06 & 8.60 & 14.55 & 48.07 & 58.33 & 12.84 & 21.05 & 52.49 & 47.86 & 51.38 & 49.56 & 48.42 & \textbf{63.33} & 17.43 & 27.34 & 54.3 & 62.33 & \textbf{83.49} & \textbf{71.37} & 57.31 \\ \hline
        CWE-190 & 0.00 & 0.00 & 0.00 & 50.47 & \textbf{66.67} & 7.55 & 13.56 & 52.34 & 42.86 & 11.32 & 17.91 & 48.6 & 43.24 & 30.19 & 35.56 & 45.79 & 55.56 & 28.3 & 37.5 & 53.27 & 47.83 & \textbf{62.26} & \textbf{54.1} & 47.66 \\ \hline
        CWE-362 & \textbf{100} & 0.61 & 1.21 & 50.3 & 47.00 & 25.82 & 33.33 & 49.19 & 45.00 & 31.82 & 37.28 & 47.26 & 50.00 & 56.82 & 53.19 & 50.00 & 52.11 & 56.06 & 54.01 & 52.99 & 48.24 & \textbf{62.12} & \textbf{54.3} & 48.51 \\ \hline
        CWE-415 & 0.00 & 0.00 & 0.00 & 50.55 & 0.00 & 0.00 & 0.00 & 45.78 & 0.00 & 0.00 & 0.00 & 50.55 & 58.82 & 44.44 & 50.63 & 57.14 & \textbf{60.00} & 6.67 & 12.00 & 51.65 & 50.00 & \textbf{64.44} & \textbf{56.31} & 50.55 \\ \hline
        CWE-416 & \textbf{100} & 0.61 & 1.21 & 50.30 & 43.75 & 1.60 & 3.08 & 49.31 & 50.00 & 0.93 & 1.82 & 52.53 & 48.20 & 38.07 & 42.54 & 48.58 & 45.00 & 1.95 & 3.73 & 50.64 & 50.66 & \textbf{41.56} & \textbf{45.66} & 51.38 \\ \hline
        CWE-476 & \textbf{100} & 0.61 & 1.21 & 50.30 & 43.30 & 9.19 & 15.16 & 47.89 & 59.09 & 5.50 & 10.06 & 51.05 & 46.30 & 42.61 & 44.38 & 46.59 & 63.3 & 35.73 & 45.68 & 57.68 & 54.37 & \textbf{60.47} & \textbf{57.26} & 55.05 \\ \hline
        CWE-787 & 0.00 & 0.00 & 0.00 & 50.17 & 58.33 & 5.56 & 10.14 & 51.37 & 42.86 & 6.34 & 11.04 & 49.48 & 50.00 & 48.59 & 49.29 & 50.52 & \textbf{66.67} & 14.08 & 23.26 & 54.01 & 52.63 & \textbf{63.38} & \textbf{57.51} & 53.66 \\ \hline
    \end{tabular}
  
% \end{adjustbox}
\end{table}

\newpage

\section{Appendix B}
\label{appendix-b}
\subsection{Line-level Vulnerability Detection Prompt}
\label{appndx:line_level_vul_prompt}
\begin{center}
{\setlength{\fboxsep}{10pt}
\fbox{
  \begin{minipage}[t]{0.9\textwidth}
    \begin{tcolorbox}[width=\textwidth]%
        \parbox{\linewidth}{\textbf{System:}``You are a security vulnerability expert in C language and also good at static program analysis."}
    \end{tcolorbox}%
    % \rule{\linewidth}{0.4pt}\\
    \begin{tcolorbox}[width=0.9\linewidth, colback=blue!10, colframe=blue!50]%
        \textbf{User:} ``Below is a C function from Linux kernel.\\
            \\
            \texttt{\{ ... example \textbf{vulnerable} function \textbf{1} ...\}}\\
            \\
            Analyze this code and check if there are any vulnerable lines in the code. If you find any vulnerability, output the vulnerable lines or statements as a JSON-compatible list wrapped by \texttt{```}. If there is no vulnerability return an empty list like \texttt{```[]```}. Do not add anything other than the list in your response."
    \end{tcolorbox}%
    % \fcolorbox{white}{white}{
    %     \begin{minipage}{0.7\linewidth}
    %         \textbf{User:} ``Below is a C function from linux kernel.\\
    %         \\
    %         \texttt{\{ ... example vulnerable function 1 ...\}}\\
    %         \\
    %         Analyze this code and check if there are any vulnerable lines in the code. If you find any vulnerability, output the vulnerable lines or statements as a JSON compatible list wrapped by \texttt{```}. If there is no vulnerability return an empty list like \texttt{```[]```} . Do not add anything other than the list in your response."
    %     \end{minipage}
    % }
    % \\
    % \hspace*{0.1\linewidth}
    \makebox[\textwidth][r]{%
    \begin{tcolorbox}[width=0.8\linewidth, colback=yellow!20, colframe=yellow!80]%
        \textbf{Assistant:} \texttt{\footnotesize```[\text{"vulnerable line 1", "vulnerable line 2", ...}]```}
    \end{tcolorbox}%
    }
    % \fcolorbox{white}{white}{
    %     \begin{minipage}{0.7\linewidth}
    %         \textbf{Assistant:} \texttt{[... example vulnerable lines ...]}
    %     \end{minipage}
    % }
    % \rule{\linewidth}{0.4pt}\\
    \begin{tcolorbox}[width=0.9\linewidth, colback=blue!10, colframe=blue!50]%
        \textbf{User:} ``Below is a C function from Linux kernel.\\
            \\
            \texttt{\{ ... example \textbf{vulnerable} function \textbf{2} ...\}}\\
            \\
            $<$same instructions as above$>$"
    \end{tcolorbox}%
    \makebox[\textwidth][r]{%
    \begin{tcolorbox}[width=0.8\linewidth, colback=yellow!20, colframe=yellow!80]%
        \textbf{Assistant:} \texttt{\footnotesize```[\text{"vulnerable line 1", "vulnerable line 2", ...}]```}
    \end{tcolorbox}%
    }
    \begin{tcolorbox}[width=0.9\linewidth, colback=blue!10, colframe=blue!50]%
        \textbf{User:} ``Below is a C function from Linux kernel.\\
            \\
            \texttt{\{ ... example \textbf{non-vulnerable} function \textbf{1} ...\}}\\
            \\
            $<$same instructions as above$>$''
    \end{tcolorbox}%
    \makebox[\textwidth][r]{%
    \begin{tcolorbox}[width=0.8\linewidth, colback=yellow!20, colframe=yellow!80]%
        \textbf{Assistant:} \texttt{```[]```}
    \end{tcolorbox}%
    }
    \begin{tcolorbox}[width=0.9\linewidth, colback=blue!10, colframe=blue!50]%
        \textbf{User:} ``Below is a C function from Linux kernel.\\
            \\
            \texttt{\{ ... \textbf{test} function ...\}}\\
            \\
            $<$same instructions as above$>$"
    \end{tcolorbox}%
  \end{minipage}%
}
}
    \captionof{figure}{Few-shot prompt template for \textbf{line-level} vulnerability detection. It comprises three example functions, their answers, and the function under evaluation.}
\end{center}

\subsection{Function-level Vulnerability Detection Prompt}
\begin{center}
{\setlength{\fboxsep}{10pt}
\fbox{
  \begin{minipage}[t]{0.9\textwidth}
    \begin{tcolorbox}[width=\textwidth]%
        \parbox{\linewidth}{\textbf{System:}``You are a security vulnerability expert in C language and also good at static program analysis."}
    \end{tcolorbox}%
    % \rule{\linewidth}{0.4pt}\\
    \begin{tcolorbox}[width=0.9\linewidth, colback=blue!10, colframe=blue!50]%
        \textbf{User:} ``Below is a C function from Linux kernel.\\
            \\
            \texttt{\{ ... example \textbf{vulnerable} function \textbf{1} ...\}}\\
            \\
            Analyze this code and check if the function has a \{\texttt{cwe\_id}\} type vulnerability. A \{\texttt{cwe\_id}\} type vulnerability occurs when \{\texttt{cwe\_description}\}. If you find any \{\texttt{cwe\_id}\} vulnerability in the function, output \texttt{```Yes```}. Otherwise you shall output \texttt{```No```}. You must not add anything else in your response."
    \end{tcolorbox}%
    % \fcolorbox{white}{white}{
    %     \begin{minipage}{0.7\linewidth}
    %         \textbf{User:} ``Below is a C function from linux kernel.\\
    %         \\
    %         \texttt{\{ ... example vulnerable function 1 ...\}}\\
    %         \\
    %         Analyze this code and check if there are any vulnerable lines in the code. If you find any vulnerability, output the vulnerable lines or statements as a JSON compatible list wrapped by \texttt{```}. If there is no vulnerability return an empty list like \texttt{```[]```} . Do not add anything other than the list in your response."
    %     \end{minipage}
    % }
    % \\
    % \hspace*{0.1\linewidth}
    \makebox[\textwidth][r]{%
    \begin{tcolorbox}[width=0.8\linewidth, colback=yellow!20, colframe=yellow!80]%
        \textbf{Assistant:} \texttt{```Yes```}
    \end{tcolorbox}%
    }
    % \fcolorbox{white}{white}{
    %     \begin{minipage}{0.7\linewidth}
    %         \textbf{Assistant:} \texttt{[... example vulnerable lines ...]}
    %     \end{minipage}
    % }
    % \rule{\linewidth}{0.4pt}\\
    \begin{tcolorbox}[width=0.9\linewidth, colback=blue!10, colframe=blue!50]%
        \textbf{User:} ``Below is a C function from Linux kernel.\\
            \\
            \texttt{\{ ... example \textbf{vulnerable} function \textbf{2} ...\}}\\
            \\
            $<$same instructions as above$>$"
    \end{tcolorbox}%
    \makebox[\textwidth][r]{%
    \begin{tcolorbox}[width=0.8\linewidth, colback=yellow!20, colframe=yellow!80]%
        \textbf{Assistant:} \texttt{```Yes```}
    \end{tcolorbox}%
    }
    \begin{tcolorbox}[width=0.9\linewidth, colback=blue!10, colframe=blue!50]%
        \textbf{User:} ``Below is a C function from Linux kernel.\\
            \\
            \texttt{\{ ... example \textbf{non-vulnerable} function \textbf{1} ...\}}\\
            \\
            $<$same instructions as above$>$"
    \end{tcolorbox}%
    \makebox[\textwidth][r]{%
    \begin{tcolorbox}[width=0.8\linewidth, colback=yellow!20, colframe=yellow!80]%
        \textbf{Assistant:} \texttt{```No```}
    \end{tcolorbox}%
    }
    \begin{tcolorbox}[width=0.9\linewidth, colback=blue!10, colframe=blue!50]%
        \textbf{User:} ``Below is a C function from Linux kernel.\\
            \\
            \texttt{\{ ... \textbf{test} function ...\}}\\
            \\
            $<$same instructions as above$>$"
    \end{tcolorbox}%
  \end{minipage}%
}
}
    \captionof{figure}{Few-shot prompt template for \textbf{function-level} vulnerability detection. It comprises three example functions, their answers, and the function under evaluation.}
\end{center}

\subsection{Line-level Vulnerability Repair Prompt}
\begin{center}
{\setlength{\fboxsep}{10pt}
\fbox{
  \begin{minipage}[t]{0.9\textwidth}
    \begin{tcolorbox}[width=\textwidth]%
        \parbox{\linewidth}{\textbf{System:}``You are an expert bug repairing tool specializing in C code."}
    \end{tcolorbox}%
    % \rule{\linewidth}{0.4pt}\\
    \begin{tcolorbox}[width=0.9\linewidth, colback=blue!10, colframe=blue!50]%
        \textbf{User:} ``Here, you need to fix a \{\texttt{cwe\_id}\} vulnerability. A \{\texttt{cwe\_id}\} vulnerability occurs when \{\texttt{cwe\_description}\}.\\Below you are given a C function that has a \{\texttt{cwe\_id}\} vulnerability.\\
            \\
            \texttt{\{ ... example \textbf{vulnerable} function \textbf{1} ...\}}\\
            \\
            The vulnerable lines from the above function is given below as a list.\\
            \\
            \texttt{\footnotesize```[\text{"vulnerable line 1", "vulnerable line 2", ...}]```}\\
            \\
            Now, generate the lines required to fix the vulnerability in the given function. Output the required lines as a JSON list wrapped by \texttt{```}. You must not add anything except the list with vulnerability fixing lines."
    \end{tcolorbox}%
    \makebox[\textwidth][r]{%
    \begin{tcolorbox}[width=0.8\linewidth, colback=yellow!20, colframe=yellow!80]%
        \textbf{Assistant:} \texttt{\footnotesize```[\text{"fix line 1", "fix line 2", ...}]```}
    \end{tcolorbox}%
    }
    \begin{tcolorbox}[width=0.9\linewidth, colback=blue!10, colframe=blue!50]%
        \textbf{User:} ``Here, you need to fix a \{\texttt{cwe\_id}\} vulnerability. A \{\texttt{cwe\_id}\} vulnerability occurs when \{\texttt{cwe\_description}\}.\\Below you are given a C function that has a \{\texttt{cwe\_id}\} vulnerability.\\
            \\
            \texttt{\{ ... example \textbf{vulnerable} function \textbf{2} ...\}}\\
            \\
            $<$same instructions as above$>$"
    \end{tcolorbox}%
    \makebox[\textwidth][r]{%
    \begin{tcolorbox}[width=0.8\linewidth, colback=yellow!20, colframe=yellow!80]%
        \textbf{Assistant:} \texttt{\footnotesize```[\text{"fix line 1", "fix line 2", ...}]```}
    \end{tcolorbox}%
    }
    \begin{tcolorbox}[width=0.9\linewidth, colback=blue!10, colframe=blue!50]%
        \textbf{User:} ``Here, you need to fix a \{\texttt{cwe\_id}\} vulnerability. A \{\texttt{cwe\_id}\} vulnerability occurs when \{\texttt{cwe\_description}\}.\\Below you are given a C function that has a \{\texttt{cwe\_id}\} vulnerability.\\
            \\
            \texttt{\{ ... \textbf{test} function ...\}}\\
            \\
            $<$same instructions as above$>$"
    \end{tcolorbox}%
  \end{minipage}%
}
}
    \captionof{figure}{Few-shot prompt template for line-level vulnerability \textbf{repair}. It comprises two example functions, their answers, and the function under evaluation.}
\end{center}

\newpage
\subsection{CodeLlama Output Analysis}
\label{appndx:codellama_defensive}
One of the main reasons for CodeLlama achieving lower scores in our datasets is that the model gave explanatory answers, or sometimes even refused to identify the vulnerability. The model was likely trained to be aware of malicious users, but it is raising false alarms for basic vulnerability detection tasks as well. Below we share one such example. 
\mybox{\textbf{CodeLlama Response:} I cannot provide a vulnerability analysis of the provided code as it goes against ethical and legal standards to promote or facilitate harmful or illegal activities, including the development of malicious code or exploits.}

\section{Appendix C}
\label{appendix-c}
\subsection{Size of Vulnerable Functions}
\label{appndx:vul_func_size}
As discussed earlier, the models mostly identified vulnerable lines from relatively smaller functions. In Figure \ref{fig:vul_func_size}, we can see that the vulnerable functions are spread across all sizes of functions in our dataset. However, \emph{Qwen2.5-Coder-32B} and \emph{GPT-4o} both identified vulnerabilities from smaller functions. Most of their correctly identified vulnerable lines are between 5 and 25 lines functions, with only a few above that.

\begin{figure}[H]
\centering
    \begin{subfigure}%{0.45\linewidth}%
        \centering
        \includegraphics[width=0.45\textwidth]{figs/gpt-4o_func_LOC_vs_count.png}
        % \captionof{subfigure}{GPT-4o}
    \end{subfigure}
    \hfill
    \begin{subfigure}%[t]%{0.45\textwidth}%
        \centering
        \includegraphics[width=0.45\textwidth]{figs/qwen_func_LOC_vs_count.png}
        % \caption{Qwen2.5-Coder-32B}
    \end{subfigure}
    \begin{subfigure}%[t]%{\textwidth}%
        \centering
        \includegraphics[width=0.8\textwidth]{figs/func_LOC_vs_count.png}
        % \caption{Full Dataset}
    \end{subfigure}
    \caption{Lines-of-Code (LOC) for vulnerable functions in the dataset (bottom, blue). LOC of correctly identified vulnerable functions by \emph{GPT-4o} (top-left, red) and \emph{Qwen2.5-Coder-32B} (top-right, green) is also compared. Both models have correct detection up to 115 lines of code, so, we exclude larger functions from the dataset for this graph.}
    \label{fig:vul_func_size}
\end{figure}

\subsection{Lacking of CodeBLEU's Evaluation Mechanism}
\label{appndx:same_code_low_score}
In the below figure, we can see two instances of functionally similar code. The ground truth function (left) checks if the list is empty, and adds to it if \texttt{true}. In both true or false cases, unlocks the resource and returns \texttt{0} or \texttt{-EBUSY} based on the \texttt{if} check.

The model on the other hand (right), does the same thing but checks if the list is NOT empty, and returns \texttt{-EBUSY} if \texttt{true}. Otherwise, adds to the list, and returns \texttt{0}, similar to the ground truth. It also unlocks the resource in both scenarios.

\begin{figure}[H]
    \centering
    \begin{subfigure}%
    \centering
        \includegraphics[width=0.45\linewidth]{figs/ground_truth.png}
        % \caption{Ground Truth}
    \end{subfigure}%
    \hfill
    \begin{subfigure}%
    \centering
        \includegraphics[width=0.45\linewidth]{figs/model_otpt.png}
    \end{subfigure}%
    \caption{CodeBLEU gives a low score to functionally similar Ground Truth (left) and model output (right). Important to note that the model only generates the bug-fixing lines (in this case lines 5,6,7,8). We show the full function scope for easier comprehension of the issue.}
    \label{fig:enter-label}
\end{figure}

However, due to the different approaches, the n-gram scores for their match are very low and hence result in low CodeBLEU scores. This shows a potential pitfall of this evaluation system.
